# Supplementary material for: Co-Supervised Learning: Improving Weak-to-Strong Generalization with Hierarchical Mixture of Experts
Source: arXiv:2402.15505 source file (2024-02-23)
Supplement: Supplementary file 1 [file appendix.tex]

% \begin{table}[th]
% \centering
% \small
% \caption{
%     Quantitative results of sim-to-real transfer from ORCA simulations to 25\% of the ETH-UCY dataset.
% }
% \vskip 0.2in
% \resizebox{\linewidth}{!}{%
%     \begin{tabular}{l c c c c c c c c c c c}
%     \toprule
%     25\% & ETH & HOTEL & UNIV & ZARA1 & ZARA2 & AVG \\            
%     \midrule
%     AutoBots~\citep{girgisLatentVariableSequential2021} & 0.942/1.886 & 0.333/0.662 & 0.563/1.156 & 0.446/0.958 & 0.409/0.904 & 0.539/1.113\\
%     + Vanilla~\citep{liangSimAugLearningRobust2020} & 0.956/1.893 & 0.352/0.698 & \textbf{0.537/1.143} & 0.439/0.969 & 0.426/0.935 & 0.542/1.128 \\
%     + Augment~\citep{roelofsCausalAgentsRobustnessBenchmark2022a} & 0.942/1.867 & 0.359/0.722 & 0.544/1.152 & 0.441/0.971 & 0.409/0.922 & 0.539/1.127 \\
%     + Contrast (ours) & 0.938/1.885 & 0.320/0.616 & 0.565/1.187 & 0.450/0.971 & 0.386/0.821 & 0.532/1.096 \\
%     + Ranking (ours) & \textbf{0.906/1.814} & \textbf{0.307/0.582} & 0.556/1.157& \textbf{0.435/0.942} & \textbf{0.376/0.819} & \textbf{0.516/1.063} \\
%     \bottomrule
%     \end{tabular}        
% }
% \label{tab:ethucy25}
% \vskip -0.2in
% \end{table}


% \begin{table}[th]
% \centering
% \small
% \caption{Quantitative results of sim-to-real transfer from ORCA simulations to 50\% of the ETH-UCY dataset.
% }
% \vskip 0.2in
% \resizebox{\linewidth}{!}{%
%     \begin{tabular}{l c c c c c c c c c c c}
%     \toprule
%     50\% & ETH & HOTEL & UNIV & ZARA1 & ZARA2 & AVG \\            
%     \midrule
%     AutoBots~\citep{girgisLatentVariableSequential2021} & 0.940/1.883 & 0.326/0.612 & 0.566/1.197 & 0.434/0.945 & 0.358/0.787 & 0.525/1.085\\
%     + Vanilla~\citep{liangSimAugLearningRobust2020} & 0.923/1.913 & 0.342/0.661 & \textbf{0.535/1.141} & 0.430/0.954 & 0.383/0.886 & 0.523/1.111 \\
%     + Augment~\citep{roelofsCausalAgentsRobustnessBenchmark2022a} & 0.937/1.885 & 0.340/0.660 & 0.535/1.146 & 0.424/0.938 & 0.377/0.878 & 0.523/1.101 \\
%     + Contrast (ours) & 0.935/1.870 & 0.344/0.667 & 0.554/1.148 & 0.422/0.913 & 0.346/0.772 & 0.520/1.074 \\
%     + Ranking (ours) & \textbf{0.903/1.810} & \textbf{0.300/0.566} & 0.543/1.146& \textbf{0.420/0.911} & \textbf{0.331/0.725} & \textbf{0.499/1.029} \\
%     \bottomrule
%     \end{tabular}        
% }
% \label{tab:ethucy50}
% \vskip -0.2in
% \end{table}



% \begin{table}[th]
% \centering
% \small
% \caption{Quantitative results of sim-to-real transfer from ORCA simulations to 100\% of the ETH-UCY dataset.
% }
% \vskip 0.2in
% \resizebox{\linewidth}{!}{%
%     \begin{tabular}{l c c c c c c c c c c c}
%     \toprule
%     100\% & ETH & HOTEL & UNIV & ZARA1 & ZARA2 & AVG \\            
%     \midrule
%     AutoBots~\citep{girgisLatentVariableSequential2021}             & 0.938/1.916 & 0.334/0.678 & 0.550/1.152 & 0.420/0.916 & 0.343/0.787 & 0.517/1.090\\
%     + Vanilla~\citep{liangSimAugLearningRobust2020}                 & 0.923/1.913 & 0.331/0.638 & 0.527/1.133 & 0.410/0.907 & 0.346/0.783 & 0.507/1.075 \\
%     + Augment~\citep{roelofsCausalAgentsRobustnessBenchmark2022a}   & 0.938/1.878 & 0.332/0.635 & \textbf{0.518/1.141} & \textbf{0.403/0.890} & 0.348/0.796 & 0.508/1.068 \\
%     + Contrast (ours)                                               & 0.930/1.896 & 0.321/0.605 & 0.538/1.154 & 0.412/0.899 & 0.345/0.791 & 0.509/1.069 \\
%     + Ranking (ours) & \textbf{0.900/1.780} & \textbf{0.296/0.556} & 0.539/1.148& 0.408/0.889 & \textbf{0.325/0.715} & \textbf{0.494/1.018} \\
%     \bottomrule
%     \end{tabular}        
% }
% \label{tab:ethucy100}
% \vskip -0.2in
% \end{table}

% \section{Additional Results} \label{appendix:results}

% In addition to the aggregated results presented in~\cref{fig:ethucy}, we summarize an in-depth breakdown of the sim-to-real transfer results in~\cref{tab:ethucy25,tab:ethucy50,tab:ethucy100}.
% Across all evaluated settings, our ranking-based causal transfer consistently achieves superior prediction accuracy compared to the AutoBots baseline. Notably, it outpaces the standard sim-to-real method~\citep{liangSimAugLearningRobust2020} in four out of the five subsets, with the sole exception in the UNIV subset.
% We conjecture that this exception might be attributed to the high similarity between the ORCA simulation and UNIV dataset.

% To assess the stability of the ranking-based method, we conducted experiments using three different random seeds, as illustrated in~\cref{fig:eth_ucy_ade,fig:eth_ucy_fde}. The results show that the ranking-based method consistently outperforms the vanilla model across all subsets of the ETH-UCY dataset. Furthermore, the ranking-based method typically yields smaller standard deviations, indicating more consistent performance.

% Furthermore, as summarized in~\cref{tab:ethucysota}, AutoBots stands as one of the state-of-the-art models for multi-agent trajectory forecasting, leaving only marginal room for improvement on the ETH-UCY dataset.
% In spite of this, our proposed causal transfer method still offers notable improvements, resulting in comparable accuracies to EqMotion~\citep{xuEqMotionEquivariantMultiAgent2023}, the most recent model that leverages domain-specific knowledge for predictive tasks.

% Finally, we summarize the results of different methods in terms of 
% Final Displacement Error (FDE) on the OOD test sets in~\cref{fig:OOD_FDE}. Similar to ~\cref{fig:quantitative_ood}, our ranking-based method leads to the lowest prediction errors compared to the other counterparts, reaffirming its strength for boosting out-of-distribution robustness.

% \begin{table}[t]
% \centering
% \small
% \caption{Comparison between different multi-agent forecasting models on the ETH-UCY dataset. 
% Boosted by our proposed ranking-based causal transfer, the best result of AutoBots across three random seeds reaches comparable performance to the current state-of-the-art.}
% \vskip 0.2in
% \resizebox{\linewidth}{!}{%
%     \begin{tabular}{l c c c c c c c c c c c}
%     \toprule
%     Deterministic & ETH & HOTEL & UNIV & ZARA1 & ZARA2 & AVG \\            
%     \midrule
%     S-LSTM~\citep{alahiSocialLSTMHuman2016} & 1.09/2.35 & 0.79/1.76 & 0.67/1.40 & 0.47/1.00 & 0.56/1.17 & 0.72/1.54\\
%     D-LSTM~\citep{kothariHumanTrajectoryForecasting2021} & 1.05/2.10 & 0.46/0.93 & 0.57/1.25 & 0.40/0.90 & 0.37/0.89 & 0.57/1.21 \\
%     Trajectron++~\citep{salzmannTrajectronDynamicallyFeasibleTrajectory2020a} & 1.02/2.00 & 0.33/0.62 & 0.53/1.19 & 0.44/0.99 & 0.32/0.73 & 0.53/1.11 \\
%     EqMotion\citep{xuEqMotionEquivariantMultiAgent2023} & 0.96/1.92 &  \textbf{0.30}/0.58 & \textbf{0.50/1.10} & \textbf{0.39/0.86} & \textbf{0.30/0.68} & \textbf{0.49}/1.03 \\
%     AutoBots ~\citep{girgisLatentVariableSequential2021} & 0.93/1.87 & 0.32/0.65 & 0.54/1.15 & 0.42/0.91 & 0.34/0.77 & 0.51/1.07 \\
%     % AutoBots ~\citep{girgisLatentVariableSequential2021} & 0.94/1.92 & 0.33/0.68 & 0.55/1.15 & 0.42/0.92 & 0.34/0.79 & 0.52/1.09 \\
%     AutoBots + Ranking (ours) & \textbf{0.90/1.78} & \textbf{0.30/0.56} & 0.53/1.12 & 0.41/0.89 & 0.32/0.70 & \textbf{0.49/1.01} \\
%     \bottomrule
%     \end{tabular}        
% }
% \label{tab:ethucysota}
% \vskip -0.2in
% \end{table}


% % \begin{table}[t]
% % \centering
% % % \vspace{-20pt}
% % \caption{Performance of D-LSTM baseline compared with our proposed regularizers.
% % \vspace{-5pt}
% % }
% % \resizebox{1\textwidth}{!}{%
% %     \begin{tabular}{l c c c c c}
% %     \toprule
% %             & ADE {$\downarrow$} & FDE {$\downarrow$} & ACE-NC {$\downarrow$} & ACE-DC {$\downarrow$} & ACE-IC {$\downarrow$}\\
% %     \midrule
% %     D-LSTM~\citep{kothariHumanTrajectoryForecasting2021} & 0.329 & 0.677 & 0.027  & 0.532 & 0.614 \\
% %     % D-LSTM + contrast & 0.334 & 0.689 & 0.027 & 0.491 & 0.429 \\
% %     D-LSTM + ranking e6 & 0.335 & 0.685 & 0.026 & 0.487 & 0.421 \\
% %     % D-LSTM + ranking e5 & 0.353 & 0.715 & 0.025 & 0.475 & 0.419\\
% %     \bottomrule
% %     \end{tabular}
% % }
% % \label{tab:D-LSTM}
% % \end{table}



% \section{Implementation Details} \label{appendix:implementation}

% \paragraph{Experiment details.}

% Our experiments are largely built upon the public code of prior work, with as few modifications as possible made for the implementations of our proposed regularizers.
% Concretely, in the robustness analysis reported in \cref{tab:baselines}, we train each model on our constructed dataset using the default hyperparameters of the corresponding baseline.
% To understand the performance of our proposed methods in \cref{subsec:synthetic}, we fine-tune the pre-trained checkpoint for 10 epochs, and evaluate the obtained model on the hold-out test set. The main hyperparameters used for training our baseline model AutoBots~\citep{girgisLatentVariableSequential2021} and the causal regularizers are listed in \cref{tab:hyper}.

% \paragraph{Simulation details.}

% Our diagnostic dataset is generated using a customized version of the Reciprocal Velocity Obstacle simulator that employs Optimal Reciprocal Collision Avoidance (ORCA) \citep{berg2011reciprocal}.
% To simulate realistic causal relationships between agents, we imposed a visibility constraint where an agent only observes other neighbors within their proximity and its \ang{210} field of view. This visibility plays a significant role in determining the influence of one agent on another. Specifically, we define a neighbor $i$ as having a {\it direct influence} on the ego agent at time step $t$ if it is visible to the ego in that time step, \ie, $\mathbbm{1}^i_t=1$.
% % Given that the simulator utilizes visible neighbors at each time-step to plan for each agent's next move, these visible neighbors exert a direct effect on the ego's trajectory.
% Additionally, we introduce a visibility window that records agents that were previously visible, facilitating the modeling of a richer spectrum of direct and indirect inter-agent influences.
% To encourage the presence of non-causal agents in dense spaces, we explicitly directed specific agents to follow others, thereby making them non-causal or indirect causal.

% \paragraph{Dataset details.}

% \cref{tab:dataset} summarize the key statistics of our diagnostic datasets, including both the in-distribution (ID) training set and the out-of-distribution (OOD) test set.
% Specifically, we consider three distinct types of OOD datasets, each deviating from the ID dataset in specific aspects, such as agent density and/or scene context.
% \begin{itemize}[nosep]
%     \item {\em ID}: The training dataset is characterized by an average of 12 pedestrians per scene, each interacting with a few others to navigate towards their goals. All the scenes are set in an open area context, allowing unrestricted movements and serving as the base environment in our experiments.
%     \item {\em OOD Density}: In our first OOD set, we retain the same context setting as the ID dataset but increase agent density. Specifically, we introduce more agents in proximity to the ego agent to intensify agent interactions. Additionally, we add agents behind the ego agent, which results in more non-causal agents. This dataset aims to test the robustness of the model in handling increased agent density.
%     \item {\em OOD Context}: The second OOD set alters the scene context from an open area to a narrow street, where pedestrians walk from one end to the other. Given that agents walking in the same direction generally do not interact, we double the number of agents in the scene, thus ensuring a similar degree of interaction complexity to the ID dataset.
%     \item {\em OOD Density+Context}: The last OOD set differs from the training one in both density and context. Here, we introduce static agents into an open area, akin to a plaza where people occasionally engage in conversations or observe their surroundings. This new type of agents, along with the increased density, presents a challenging OOD setting.
% \end{itemize}
% Exemplary animations for each data split can be found in our public repository.

% % \Ahmad{For the original dataset (In-Distribution), we design the scenarios such that on average 12 agents in the scene have close interactions with each other and most of them have to cross a few other agents to reach to their goal. As there is no special shape for this setting, we call it an open area where pedestrians can walk freely in the environment. For the Density dataset, we increased the number of agents both around the ego agent (increasing the magnitude of interactions) and behind the agent (introducing more non-causal agents). Another scene setting that we used, is an street, where pedestrians form two lines, with each line walking towards the other. Therefore the number of agents that the ego agent has effective interaction with reduces, since half the agents are behind or beside him, therefore we kept the number of agents high to have meaningful interactions. Finally, we introduced a number of static agents to the open area scene setting, making it look more like a plaza, where people could often stay and have a talk or look around. This is a new type of agent, which combined with the density of other agents in the scene, makes avoiding collisions and planning harder.} 
% % \todo{add the link to the repo for animations here.}


% \paragraph{Baseline details.}
% To the best of our knowledge, few prior work studies causally-aware representation learning in the multi-agent context.
% To examine the efficacy of our proposed methods, we consider the following three existing methods as comparative baselines.
% \begin{itemize}[nosep]
%     \item {\em Baseline}: the baseline method trains the model on the data in the target domain only, \ie, the AutoBots baseline trained on the in-distribution dataset in \cref{subsec:synthetic} or the real-world ETH-UCY dataset in \cref{subsec:s2r}.
%     \item {\em Vanilla}: the vanilla sim-to-real method combines simulated and real-world data in the training process. It adheres to a standard prediction task, with an equal mix of data from each domain in every training batch~\citep{liangSimAugLearningRobust2020}. 
%     \item {\em Augment}: the causal augmentation method is built upon the {\em Baseline} for the experiment in \cref{subsec:synthetic} or the {\em Vanilla} for the experiment in \cref{subsec:s2r}. It augments training data by randomly dropping non-causal agents based on the provided annotations~\citep{roelofsCausalAgentsRobustnessBenchmark2022a}.
% \end{itemize}




% \begin{figure}[t]
%     \vskip 0.2in
%     \centering
%     \begin{subfigure}[b]{0.375\linewidth}
%         \centering
%         \includegraphics[height=120pt]{figures/quantitative_ood_FDE_errorbar.pdf}
%     \end{subfigure}
%     \caption{Additional quantitative results of our method on the out-of-distribution test sets, as a supplement to \cref{fig:quantitative_ood}. Models trained by our method yield lower FDE. Results are averaged over five random seeds.}
%   \label{fig:OOD_FDE}
% \end{figure}

% \begin{figure}[t]
%     \centering
%     \begin{subfigure}[b]{0.45\linewidth}
%         \centering
%         \includegraphics[height=100pt]{figures/quantitative_ace_dc.pdf}
%     \end{subfigure}
%     \quad
%     \begin{subfigure}[b]{0.45\linewidth}
%         \centering
%         \includegraphics[height=100pt]{figures/quantitative_ace_ic.pdf}
%     \end{subfigure}
%     \caption{Additional quantitative results of our method on causal effect estimates, as a supplement to \cref{fig:quantitative_ace}.
%     Models trained by our method yield lower ACE-DC and ACE-ID, especially noticeable in scenarios with low-quantile ground-truth causal effects. Results are averaged over five random seeds.}.
%     \label{fig:ace}
% \end{figure}

% % Quantitaive results of our causal regularization method in comparison to the Autobots baseline~\citep{girgisLatentVariableSequential2021} and the non-causal data augmentation~\citep{roelofsCausalAgentsRobustnessBenchmark2022a} Models trained by our ranking-based method yield enhanced accuracy in estimating causal effects and more reliable predictions on out-of-distribution test sets.
% % Results are averaged over five random seeds.


% \begin{figure}[t]
%     \vskip 0.2in
%     \centering
%     % First row of subfigures
%     \begin{subfigure}[b]{0.32\linewidth}
%         \centering
%         \includegraphics[width=1.0\linewidth]{figures/ADE_HOTEL.pdf}
%         \caption{HOTEL}
%         \label{fig:ade_hotel}
%     \end{subfigure}
%     ~
%     \begin{subfigure}[b]{0.32\linewidth}
%         \centering
%         \includegraphics[width=1.0\linewidth]{figures/ADE_UNIV.pdf}
%         \caption{UNIV}
%         \label{fig:ade_univ}
%     \end{subfigure}
%     ~
%     \begin{subfigure}[b]{0.32\linewidth}
%         \centering
%         \includegraphics[width=1.0\linewidth]{figures/ADE_ETH.pdf}
%         \caption{ETH}
%         \label{fig:ade_eth}
%     \end{subfigure}
%     % Second row of subfigures
%     \begin{subfigure}[b]{0.32\linewidth}
%         \centering
%         \includegraphics[width=1.0\linewidth]{figures/ADE_ZARA1.pdf}
%         \caption{ZARA1}
%         \label{fig:ade_zara1}
%     \end{subfigure}
%     ~
%     \begin{subfigure}[b]{0.32\linewidth}
%         \centering
%         \includegraphics[width=1.0\linewidth]{figures/ADE_ZARA2.pdf}
%         \caption{ZARA2}
%         \label{fig:ade_zara2}
%     \end{subfigure}
%     ~
%     \begin{subfigure}[b]{0.32\linewidth}
%         \centering
%         \includegraphics[width=1.0\linewidth]{figures/ADE_AVG.pdf}
%         \caption{Average}
%         \label{fig:ade_avg}
%     \end{subfigure}

%     \caption{Additional results of our ranking-based causal transfer on the ETH-UCY dataset, as a supplement to \cref{fig:ethucy}.
%     The results of ADE are averaged on each subset over three random seeds.}
%     \vskip -0.2in
%     \label{fig:eth_ucy_ade}
% \end{figure}


% \begin{figure}[t]
%     \vskip 0.2in
%     \centering
%     % First row of subfigures
%     \begin{subfigure}[b]{0.32\linewidth}
%         \centering
%         \includegraphics[width=1.0\linewidth]{figures/FDE_HOTEL.pdf}
%         \caption{HOTEL}
%         \label{fig:fde_hotel}
%     \end{subfigure}
%     ~
%     \begin{subfigure}[b]{0.32\linewidth}
%         \centering
%         \includegraphics[width=1.0\linewidth]{figures/FDE_UNIV.pdf}
%         \caption{UNIV}
%         \label{fig:fde_univ}
%     \end{subfigure}
%     ~
%     \begin{subfigure}[b]{0.32\linewidth}
%         \centering
%         \includegraphics[width=1.0\linewidth]{figures/FDE_ETH.pdf}
%         \caption{ETH}
%         \label{fig:fde_eth}
%     \end{subfigure}

%     % Second row of subfigures
%     \begin{subfigure}[b]{0.32\linewidth}
%         \centering
%         \includegraphics[width=1.0\linewidth]{figures/FDE_ZARA1.pdf}
%         \caption{ZARA1}
%         \label{fig:fde_zara1}
%     \end{subfigure}
%     ~
%     \begin{subfigure}[b]{0.32\linewidth}
%         \centering
%         \includegraphics[width=1.0\linewidth]{figures/FDE_ZARA2.pdf}
%         \caption{ZARA2}
%         \label{fig:fde_zara2}
%     \end{subfigure}
%     ~
%     \begin{subfigure}[b]{0.32\linewidth}
%         \centering
%         \includegraphics[width=1.0\linewidth]{figures/FDE_AVG.pdf}
%         \caption{Average}
%         \label{fig:fde_avg}
%     \end{subfigure}

%     \caption{Additional results of our ranking-based causal transfer on the ETH-UCY dataset, as a supplement to \cref{fig:ethucy}.
%     The results of FDE are averaged on each subset over three random seeds.}
%     \vskip -0.2in
%     \label{fig:eth_ucy_fde}
% \end{figure}



% \section{Additional Discussions} \label{appendix:discussion}

% \paragraph{Counterfactual simulation.}
% Our diagnostic dataset, enabled by counterfactual simulations, offers clean annotations of causal relationships, serving as a crucial step in understanding causally-aware representation of multi-agent interactions.
% However, the realism of these simulated causal effects is still subject to some inherent limitations.
% For example, we have enforced a stringent constraint on the field of view for each agent, considering that the ego agent is usually unaffected by trailing neighbors. Such constraints could compromise the optimality of the ORCA algorithm, potentially resulting in unnatural trajectories.
% We believe that integrating more advanced simulators, \eg, CausalCity~\citep{mcduffCausalCityComplexSimulations2022}, can address these challenges and we anticipate promising outcomes along this line for future research.

% \paragraph{Multi-agent causal effects.}
% Our annotation and evaluation have been focused on the causal effect at an individual agent level, namely we remove only one agent at a time.
% Through this lens, we observe that while recent representations are already partially robust to non-causal agent removal, they tend to underestimate the effects of causal agents.
% However, it is worth noting that this is still a rather simplified and restricted setting compared to the group-level causal effects, where the collective behavior of multiple agents may have a more complex influence on the ego agent. 
% Understanding and addressing this challenge can be another exciting avenue for future research. 
% \clearpage

% \begin{table}[t]
%     \small
%     \centering
%     \caption{
%     Key hyper-parameters in our experiments.
%     }
%     % \vspace{-5pt}
%     \begin{tabular}{wl{5.2cm}|wl{1.6cm}}
%         name & value \\        
%     \specialrule{.1em}{.05em}{.05em}  
%         batch size & 16 \\
%         pre-training learning rate &  $7.5\times10^{-4}$\\
%         fine-tuning learning rate &  $2.34375\times10^{-5}$\\
%         contrastive weight $\alpha$ & 1000 \\
%         ranking weight $\alpha$ & 1000 \\
%         ranking margin $m$ & 0.001 \\
%         non-causal threshold $\epsilon$ & 0.02 \\
%         causal threshold $\eta$ & 0.1 \\
        
%     \end{tabular}
%     \label{tab:hyper}
% \end{table}

% \begin{table}[t]
% \centering
% \caption{Key statistics of our diagnostic datasets.}
% \vskip 0.2in
% \resizebox{\linewidth}{!}{%
%     \begin{tabular}{l | c | c c | c c c c}
%     \toprule
%      \multirow{2}{*}{Dataset} & \multirow{2}{*}{Context} & \multicolumn{2}{c}{Number of scenes} & \multicolumn{4}{c}{Number of agents per scene} \\ 
%  & &   train  & test & non-causal & direct causal & indirect causal & total \\
%  \midrule
%      ID & open area & 20k  & 2k & 1.31 & 8.35 & 0.48 & 12.03\\
%      OOD Density & open area & - & 2k & 9.47 & 12.27 & 2.55 & 28.98\\
%      OOD Context & street & - & 2k & 8.23 & 12.22 & 3.09 & 29.01\\
%      OOD Density+Context & plaza & - & 2k & 7.49 & 14.64 & 2.78 & 28.93\\
%     \bottomrule
%     \end{tabular}        
% }
% \begin{center}
% \label{tab:dataset}
% \vskip -0.2in
% \end{center}
% \end{table}
